# Supplementary material for: Universal Domain Adaptation in Ordinal Regression
Source: arXiv:2106.11576 source file (2021-08-25)
Supplement: Supplementary file 1 [file order_table.tex]

\begin{footnotesize}
\begin{table}[h]
\centering
\begin{tabular}{|cccccccc|}
0.  &0.67& -  &-   &0.83&  - & 0.87 & - \\
0.33&0.  & 0.6&-   &0.71&  - & 0.78 & 0.8 \\
 -  &0.4 &0.  &0.58&  - & 0.67 & -    & -  \\
-   & -  &0.42&0.  &  - &  - & 0.64 & 0.67\\
0.17& -  & -  & - &0.   &-   & 0.48  &0.61\\
-   & -  &0.33& -  &-   &  0.& 0.54 & - \\
0.13&0.22&-   &0.36&0.52&0.46&0.    &0.53\\
-   &0.2 &-   &0.33&0.39& - & 0.47  & 0.\\
\end{tabular}
\caption{Matrix of pairwise comparisons for 8 instances as input to Bradlye-Terry model.}
\label{tab:ranking}
\end{table}
\end{footnotesize}
%classes: [15, 15, 16, 16, 17, 17, 18, 18, 19, 19]
